# Supplementary material for: Classification with unknown class-conditional label noise on non-compact feature spaces
Source: arXiv:1902.05627 source file (2019-06-09)
Supplement: Supplementary file 1 [file proofOfKNNRegressionBounds.tex]

In this section we complete the proof of Theorem \ref{KNNPointwiseBoundFixedKThm}. The proof relies upon Lemmas \ref{knnEstIsCloseToItsXConditionalExpectationLemma} and \ref{closeNeighboursFocusPointLemma}, both proven in Section \ref{standardLemmasProofSec}.

\begin{proof}[Proof of Theorem \ref{KNNPointwiseBoundFixedKThm}] To prove Theorem \ref{KNNPointwiseBoundFixedKThm} we first write
\begin{align}\label{mainTriangleInequalityInProofOfKNNPointwiseBoundFixedKThmEq}
\left|\KNNest[f](x)-f(x)\right| \leq \left|\KNNest[f](x)-\conditionalExpectKNNest[f](x)\right|+\left|\conditionalExpectKNNest[f](x)-f(x)\right|,
\end{align}
and then bound the two terms on the right separately, with high probability. By Lemma \ref{knnEstIsCloseToItsXConditionalExpectationLemma}, with probability at least $1-2\delta/3$ over $\sample_f$, we have
\begin{align}\label{varBoundInProofOfKNNPointwiseBoundFixedKThmEq}
\left|\KNNest[f](x)-\conditionalExpectKNNest[f](x)\right|\leq \sqrt{\frac{\log(3/\delta)}{2k}}.
\end{align}
To bound the second term in (\ref{mainTriangleInequalityInProofOfKNNPointwiseBoundFixedKThmEq}) we first apply Lemma \ref{closeNeighboursFocusPointLemma} with $p=2k/n$ to obtain,
\begin{align*}
\Prob_{\sample_f}\left[ \rho\left(x,X_{\tau_{n,k}(x)}\right) > r_p(x)\right] \leq \exp\left(-\frac{k-1}{2}\cdot\left(1-\frac{k}{np}\right)^2\right)\leq \delta/3,
 \end{align*}
since $k \geq 8 \log(3/\delta)+1$. Now let's suppose that $\rho\left(x,X_{\tau_{n,k}(x)}\right) \leq r_p(x)$. Note that by the construction of $r_p(x)$ combined with continuity from below we have $\marginalDistribution\left(B_{r_p(x)}(x)\right)\leq p$. Thus, by using the measure-smoothness of $f$ we see that for each $q \in [k]$, 
\begin{align*}
\left|f\left(X_{\tau_{n,q}(x)}\right)-f(x)\right| &\leq \localMeasureSmoothnessFactor[x] \cdot \marginalDistribution\left(B_{\rho(x,X_{\tau_{n,q}(x)})}(x)\right)^{\measureSmoothnessExponent}  \leq \localMeasureSmoothnessFactor[x] \cdot \marginalDistribution\left(B_{\rho(x,X_{\tau_{n,k}(x)})}(x)\right)^{\measureSmoothnessExponent} \\ &  \leq \localMeasureSmoothnessFactor[x] \cdot \marginalDistribution\left(B_{r_p(x)}(x)\right)^{\measureSmoothnessExponent}  \leq  \localMeasureSmoothnessFactor[x] \cdot p^{\measureSmoothnessExponent}=  \localMeasureSmoothnessFactor[x] \cdot \left(\frac{2k}{n}\right)^{\measureSmoothnessExponent}.  
\end{align*}
Thus, whenever $\rho\left(x,X_{\tau_{n,k}(x)}\right) \leq r_p(x)$  we have
\begin{align}\label{biasBoundInProofOfKNNPointwiseBoundFixedKThmEq}
\left|\conditionalExpectKNNest[f](x)-f(x)\right|\leq \frac{1}{k} \cdot \sum_{q \in [k]}\left|f\left(X_{\tau_{n,q}(x)}\right)-f(x)\right| \leq \localMeasureSmoothnessFactor[x] \cdot \left(\frac{2k}{n}\right)^{\measureSmoothnessExponent}.  
\end{align}
Moreover, $\rho\left(x,X_{\tau_{n,k}(x)}\right) \leq r_p(x)$ (and hence  holds with probability at least $1-\delta/3$. Hence, by the union bound (\ref{biasBoundInProofOfKNNPointwiseBoundFixedKThmEq}) and (\ref{biasBoundInProofOfKNNPointwiseBoundFixedKThmEq}) hold simultaneously with probability at least $1-\delta$. Plugging inequalities (\ref{varBoundInProofOfKNNPointwiseBoundFixedKThmEq}) and (\ref{biasBoundInProofOfKNNPointwiseBoundFixedKThmEq}) back into (\ref{mainTriangleInequalityInProofOfKNNPointwiseBoundFixedKThmEq}) completes the proof of the theorem.
\end{proof}
We now deduce Corollary \ref{KNNPointwiseBoundLepskiChoiceKThm} from Theorem \ref{KNNPointwiseBoundFixedKThm}.

\begin{proof}[Proof of Corollary \ref{KNNPointwiseBoundLepskiChoiceKThm}] Take $n\in \N$, $\delta \in \left(0,1\right)$ and $n \in \N$ and let $\XFocusPoint$ be either a fixed point $x \in \suppMarginalDistribution$ or $X_j$ for some fixed $j \in [n]$. By Theorem \ref{KNNPointwiseBoundFixedKThm} with $\tilde{\delta}=2\delta/n$, combined with the union bound, the following holds simultaneously for all $k \in \left\lbrace \lceil 8 \log(3n/2\delta)+1\rceil, \cdots, \lfloor n/2 \rfloor \right\rbrace$, 
\begin{align}\label{KNNPointwiseBoundFixedKThmImpliesEq}
\left|\KNNest[f](\XFocusPoint)-f(\XFocusPoint)\right| \leq  \sqrt{\frac{\log(3n/2\delta)}{2k}}+\localMeasureSmoothnessFactor[\XFocusPoint] \cdot \left(\frac{2k}{n}\right)^{\measureSmoothnessExponent}=\frac{1}{2}\cdot \uncertaintyKNNDelta+\localMeasureSmoothnessFactor[\XFocusPoint] \cdot \left(\frac{2k}{n}\right)^{\measureSmoothnessExponent}.
\end{align}
Let $k_* =\left\lceil \frac{1}{4}\cdot \left( \frac{\log(3n/2\delta)}{\localMeasureSmoothnessFactor[\XFocusPoint]^2}\right)^{\frac{1}{2\measureSmoothnessExponent+1}} \cdot n^{\frac{2\measureSmoothnessExponent}{2\measureSmoothnessExponent+1}}\right\rceil$. We may assume without loss of generality that $ 6\sqrt{2} \cdot \localMeasureSmoothnessFactor[\XFocusPoint]^{\frac{1}{2\measureSmoothnessExponent+1}} \cdot \left( \frac{\log(3n/2\delta)}{n}\right)^{\frac{\measureSmoothnessExponent}{2\measureSmoothnessExponent+1}}\leq 1$, since the conclusion of the corollary is trivial otherwise. Hence, we have
\begin{align}\label{kStarBoundsInProofOfLepskiCorEq}
8 \log(3n/2\delta)+1&\leq \frac{1}{4} \cdot \left( \frac{\log(3n/2\delta)}{\localMeasureSmoothnessFactor[\XFocusPoint]^2}\right)^{\frac{1}{2\measureSmoothnessExponent+1}} \cdot n^{\frac{2\measureSmoothnessExponent}{2\measureSmoothnessExponent+1}} \leq k_*\leq \frac{1}{2} \cdot \left( \frac{\log(3n/2\delta)}{\localMeasureSmoothnessFactor[\XFocusPoint]^2}\right)^{\frac{1}{2\measureSmoothnessExponent+1}} \cdot n^{\frac{2\measureSmoothnessExponent}{2\measureSmoothnessExponent+1}}\leq \frac{n}{2}.
\end{align}
Thus,  $k_* \in \left\lbrace \lceil 8 \log(3n/2\delta)+1\rceil, \cdots, \lfloor n/2 \rfloor \right\rbrace$. It follows from the upper bound in (\ref{kStarBoundsInProofOfLepskiCorEq}) that for all $q \leq k_*$ we have 
\begin{align*}
\localMeasureSmoothnessFactor[\XFocusPoint] \cdot \left(\frac{2q}{n}\right)^{\measureSmoothnessExponent} \leq  \sqrt{\frac{\log(3n/2\delta)}{2q}}=\frac{1}{2}\cdot \uncertaintyKNNDelta[q].
\end{align*}
Thus, from (\ref{KNNPointwiseBoundFixedKThmImpliesEq}) we see that $\left|\hat{f}_{n,q}(\XFocusPoint)-f(\XFocusPoint)\right| \leq \uncertaintyKNNDelta[q]$ for all  $q \in \{ \lceil 8\log(3n/\delta)\rceil+1,\cdots, k_*$. Hence, 
\begin{align*}
f(\XFocusPoint) \in  \bigcap_{q =\lceil 8 \log(3n/2\delta)+1\rceil}^{k_*}\intervalKNNDelta[q]\left(\XFocusPoint\right)\neq \emptyset.
\end{align*}
Hence, $k_*\leq \lepskiChoiceOfK\left(\XFocusPoint\right)$. Moreover, it follows from the lower bound in (\ref{kStarBoundsInProofOfLepskiCorEq}) that for all $q \geq k_*$ we have
\begin{align*}
\uncertaintyKNNDelta[q] \leq 2\sqrt{2} \cdot \localMeasureSmoothnessFactor[\XFocusPoint]^{\frac{1}{2\measureSmoothnessExponent+1}} \cdot \left( \frac{\log(3n/2\delta)}{n}\right)^{\frac{\measureSmoothnessExponent}{2\measureSmoothnessExponent+1}}.
\end{align*}
By the construction of $\lepskiChoiceOfK\left(\XFocusPoint\right)$ and $k_*\leq \lepskiChoiceOfK\left(\XFocusPoint\right)$ we have 
\begin{align*}
\left[\hat{f}_{n,k_*}(\XFocusPoint)-\uncertaintyKNNDelta[k_*],\hat{f}_{n,k_*}(x)+\uncertaintyKNNDelta[k_*]\right] \cap \left[\hat{f}_{n,\lepskiChoiceOfK \left(\XFocusPoint\right)}(\XFocusPoint)-\uncertaintyKNNDelta[\lepskiChoiceOfK\left(\XFocusPoint\right)],\hat{f}_{n,\lepskiChoiceOfK\left(\XFocusPoint\right)}(\XFocusPoint)+\uncertaintyKNNDelta[\lepskiChoiceOfK\left(\XFocusPoint\right)]\right] \neq \emptyset.
\end{align*}
Hence, given that  $\KNNLepskiEst[f](\XFocusPoint)=\KNNest[f](\XFocusPoint)$ with $k=\lepskiChoiceOfK\left(\XFocusPoint\right)$, we have
\begin{align*}
\left| \KNNLepskiEst[f]\left(\XFocusPoint\right)-\hat{f}_{n,k_*}\left(\XFocusPoint\right)\right| \leq \uncertaintyKNNDelta[k_*]+\uncertaintyKNNDelta[\lepskiChoiceOfK\left(\XFocusPoint\right)] \leq 4\sqrt{2} \cdot \localMeasureSmoothnessFactor[\XFocusPoint]^{\frac{1}{2\measureSmoothnessExponent+1}} \cdot \left( \frac{\log(3n/2\delta)}{n}\right)^{\frac{\measureSmoothnessExponent}{2\measureSmoothnessExponent+1}}.
\end{align*}
In addition, we have $\left|\hat{f}_{n,k_*}(\XFocusPoint)-f(\XFocusPoint)\right| \leq \uncertaintyKNNDelta[k_*] \leq 2\sqrt{2} \cdot \localMeasureSmoothnessFactor[\XFocusPoint]^{\frac{1}{2\measureSmoothnessExponent+1}} \cdot \left( \frac{\log(3n/2\delta)}{n}\right)^{\frac{\measureSmoothnessExponent}{2\measureSmoothnessExponent+1}}$. Thus, by the triangle inequality we have
\begin{align*}
\left| \KNNLepskiEst[f](\XFocusPoint)-f(\XFocusPoint)\right| &\leq \left| \KNNLepskiEst[f](\XFocusPoint)-\hat{f}_{n,k_*}(\XFocusPoint)\right| +\left|\hat{f}_{n,k_*}(\XFocusPoint)-f(\XFocusPoint)\right| \\ &\leq 6\sqrt{2} \cdot \localMeasureSmoothnessFactor[x]^{\frac{1}{2\measureSmoothnessExponent+1}} \cdot \left( \frac{\log(3n/2\delta)}{n}\right)^{\frac{\measureSmoothnessExponent}{2\measureSmoothnessExponent+1}}.
\end{align*}
This completes the proof of the corollary.
\end{proof}
