# Supplementary material for: Classification with unknown class-conditional label noise on non-compact feature spaces
Source: arXiv:1902.05627 source file (2019-06-09)
Supplement: Supplementary file 2 [file proofOfLowerConfidenceBoundsLemma.tex]

\begin{proof}[Proof of Lemma \ref{klLBIsWellBehavedForNonUniformMaxLemma}]
For each $(i,k) \in [n]$ we take $\xi_{i,k}^{+},\xi_{i,k}^{-}>0$ so that  
\begin{align*}
k \cdot \KL\left(\conditionalExpectKNNest[f](X_i)+\xi_{i,k}^{+},\conditionalExpectKNNest[f](X_i)\right)  =\log((2n)^2/\delta)\hspace{5mm}\text{\&}\hspace{5mm} k \cdot \KL\left(\conditionalExpectKNNest[f](X_i)-\xi_{i,k}^{-},\conditionalExpectKNNest[f](X_i)\right)  =\log((2n)^2/\delta).
\end{align*}
By Lemma \ref{knnEstIsCloseToItsXConditionalExpectationLemma} the following holds simultaneously for all $(i,k) \in [n]^2$, with probability at least $1-\delta/2$ over $\sample_f$,
\begin{align*}
\conditionalExpectKNNest[f](X_i)-\xi_{i,k}^{-}\leq \KNNest[f](X_i)\leq \conditionalExpectKNNest[f](X_i)+\xi_{i,k}^{+}.
\end{align*}
Suppose for a contradiction that $\KLLowerBoundKNN[f](X_i)>\conditionalExpectKNNest[f](X_i)$. It then follows from the construction of $\KLLowerBoundKNN[f](X_i)$ that $k \cdot \KL\left(\KNNest[f](X_i),\conditionalExpectKNNest[f](X_i)\right)  >\log((2n)^2/\delta)$. Moreover, we also have
\begin{align*}
\conditionalExpectKNNest[f](X_i)<\KLLowerBoundKNN[f](X_i) \leq \KNNest[f](X_i) \leq \conditionalExpectKNNest[f](X_i)+\xi_{i,k}^{+}.
\end{align*}
Hence, we can deduce the following contradiction to the definition of $\xi_{i,k}^{+}$,
\begin{align*}
k \cdot \KL\left(\conditionalExpectKNNest[f](X_i)+\xi_{i,k}^{+},\conditionalExpectKNNest[f](X_i)\right) \geq k \cdot \KL\left(\KNNest[f](X_i),\conditionalExpectKNNest[f](X_i)\right)  >\log((2n)^2/\delta).
\end{align*}
Hence, we have $\KLLowerBoundKNN[f](X_i)\leq\conditionalExpectKNNest[f](X_i)$. Now by the definition of $\KLLowerBoundKNN[f](X_i)$ combined with Pinsker's inequality we have
\begin{align*}
\left|\KLLowerBoundKNN[f](X_i)-\KNNest[f](X_i)\right|\leq \sqrt{\frac{1}{2}\cdot \KL\left(\KNNest[f](X_i),\KNNest[f](X_i)\right)}= \sqrt{\log((2n)^2/\delta)/(2k)}.
\end{align*}
Similarly, given the definition of $\xi_{i,k}^{-},\xi_{i,k}^{+}$ combined with Pinsker's inequality we have $\max\{\xi_{i,k}^{-},\xi_{i,k}^{+}\}\leq \sqrt{\log((2n)^2/\delta)/(2k)}$. Hence, we have
\begin{align*}
\left|\KLLowerBoundKNN[f](X_i)-\conditionalExpectKNNest[f](X_i)\right|\leq \left|\KLLowerBoundKNN[f](X_i)-\KNNest[f](X_i)\right|+\left|\KNNest[f](X_i)-\conditionalExpectKNNest[f](X_i)\right| \leq \sqrt{2\log((2n)^2/\delta)/k}.
\end{align*}
This completes the proof of the lemma.
\end{proof}
