# Supplementary material for: Classification with unknown class-conditional label noise on non-compact feature spaces
Source: arXiv:1902.05627 source file (2019-06-09)
Supplement: Supplementary file 3 [file standardLemmas.tex]

In this section we prove several supporting lemmas. Recall that we have a sample $\sample_f=\left\lbrace \left(X_i,Z_i\right)\right\rbrace_{i \in [n]}$.  For the purposes of the proof we let $\Xsample = \left\lbrace X_i\right\rbrace_{i \in [n]}$ and $\Zsample=\left\lbrace Z_i\right\rbrace_{i \in [n]}$. We also define $\conditionalExpectKNNest[f](x)=\E_{\Zsample|\Xsample}\left[\KNNest[f](x)\right] =\frac{1}{k} \cdot \sum_{q \in [k]}f\left(X_{\tau_{n,q}(x)}\right)$ and  $r_p(x) = \inf\left\lbrace r>0: \marginalDistribution\left(B_r(x)\right)\geq p\right\rbrace$.

 \begin{restatable}{lemma}{knnEstIsCloseToItsXConditionalExpectationLemma}\label{knnEstIsCloseToItsXConditionalExpectationLemma} Suppose that $\XFocusPoint$ is either a fixed point $x \in \suppMarginalDistribution$ or $X_j$ for some fixed $j \in [n]$. Given any $n\in \N$, $k \in [n]$ and $\xi>0$ we have
\begin{align*}
\Prob_{\Zsample|\Xsample}\left[ \KNNest[f](\XFocusPoint)\leq \conditionalExpectKNNest[f](\XFocusPoint)+\xi \right]&\leq \exp\left(- k \cdot \KL\left(\conditionalExpectKNNest[f](\XFocusPoint)+\xi,\conditionalExpectKNNest[f](\XFocusPoint)\right) \right) \leq \exp\left(-2k \cdot \xi^2\right),\\ 
\Prob_{\Zsample|\Xsample}\left[ \KNNest[f](\XFocusPoint)\geq \conditionalExpectKNNest[f](\XFocusPoint)-\xi \right]&\leq \exp\left(- k \cdot \KL\left(\conditionalExpectKNNest[f](\XFocusPoint)-\xi,\conditionalExpectKNNest[f](\XFocusPoint)\right) \right) \leq \exp\left(-2k \cdot \xi^2\right).
\end{align*}
 \end{restatable}
\begin{proof}[Proof of Lemma \ref{knnEstIsCloseToItsXConditionalExpectationLemma}] Note that $\XFocusPoint$ is a deterministic function of $\Xsample=\left\lbrace X_i \right\rbrace_{i \in [n]}$. By construction we have $\KNNest[f](\XFocusPoint) = \frac{1}{k} \cdot \sum_{q \in [k]}Z_{\tau_{n,q}(\XFocusPoint)}$. Moreover, for each $q \in [k]$, $Z_{\tau_{n,q}(\XFocusPoint)}$ is a random variable in $[0,1]$ with conditional expectation (given $\Xsample$) equal to $\E_{\Zsample|\Xsample}\left[Z_{\tau_{n,q}(\XFocusPoint)}\right] = f\left(X_{\tau_{n,q}(\XFocusPoint)}\right)$. Hence, the inequalities follow from Chernoff bounds \cite{boucheron2013concentration} combined with Pinsker's inequality.
\end{proof}

We now prove Lemma \ref{closeNeighboursFixedPointLemma} and then deduce Lemma \ref{closeNeighboursFocusPointLemma}.

\closeNeighboursFixedPointLemma*

\begin{proof}[Proof of Lemma \ref{closeNeighboursFixedPointLemma}]
Take $r>r_p(x)$, so $\mu\left(B_r(x)\right) \geq p$. Note that $\rho\left(x,X_{\tau_{n,k}(x)}\right) \geq r$ if and only if $\sum_{i\in [n]}\mathds{1}_{\{X_i \in B_r(x)\}}<k$. Moreover, taking 
\begin{align*}
\tilde{p}= \frac{1}{n}\sum_{i\in [n]}\E\left[\one_{\{X_i \in B_r(x)\}}\right]=\mu\left(B_r(x)\right) \geq p
\end{align*}
implies $k \leq (1-\epsilon) n \tilde{p}\leq n \tilde{p}$ where $\epsilon = 1-{k}/{(np)}$. Thus, by the multiplicative Chernoff bound (\cite{mitzenmacher2005probability}) we have,
\begin{align*}
\Prob^n\left[\rho\left(x,X_{\tau_{n,k}(x)}\right) \geq r\right] &\leq \Prob\left[\sum_{i\in [n]}\mathds{1}_{\{X_i \in B_r(x)\}}<k\right]\\
&\leq \Prob\left[\sum_{i\in [n]}\mathds{1}_{\{X_i \in B_r(x)\}}< (1-\epsilon)n\tilde{p}\right]\\
& \leq \exp(-n\tilde{p} \cdot \epsilon^2/2) \leq \exp(-k\cdot \epsilon^2/2).
\end{align*}
Since the above inequality holds for all $r>r_p(x)$, the lemma follows by continuity.
\end{proof}

\begin{restatable}{lemma}{closeNeighboursFocusPointLemma}\label{closeNeighboursFocusPointLemma} Suppose that $\XFocusPoint$ is either a fixed point $x \in \suppMarginalDistribution$ or $X_j$ for some fixed index $j \in [n]$. Given $k \in [n]$ and $p\in [k/n,1]$ we have $\Prob_{\sample}\left[ \rho\left(\XFocusPoint,X_{\tau_{n,k}(\XFocusPoint)}\right) > r_p(\XFocusPoint)\right] \leq \exp\left(-\frac{k-1}{2}\cdot\left(1-\frac{k}{np}\right)^2\right)$.
\end{restatable}

\begin{proof}[Proof of Lemma \ref{closeNeighboursFocusPointLemma}] Either (a) $\XFocusPoint= x$ for some fixed point $x \in \suppMarginalDistribution$ or (b) $\XFocusPoint= X_j$ for some fixed $j \in [n]$. In case (a) the bound in Lemma \ref{closeNeighboursFocusPointLemma} follows immediately from Lemma \ref{closeNeighboursFixedPointLemma}. In case (b), since the data is i.i.d. we may assume without loss generality that $j=n$. Applying Lemma \ref{closeNeighboursFixedPointLemma} to $\sample_{n-1}=\left\lbrace (X_i,Z_i)\right\rbrace_{i \in [n-1]} \sim \Prob^{n-1}$, with $n-1$ in place of $n$ and $k-1$ in place of $k$, we see that for each $x \in \suppMarginalDistribution$ we have
\begin{align*}
&\Prob_{\sample_{n-1}}\left[ \sum_{i \in [n-1]}\one\left\lbrace \dist\left(x,X_i \right)\leq r_p(x)\right\rbrace  < k-1\right]=
\Prob_{\sample_{n-1}}\left[ \rho\left(x,X_{\tau_{n-1,k-1}(x)}\right) > r_p(x)\right]\\ &\leq \exp\left(-\frac{k-1}{2}\cdot\left(1-\frac{k-1}{(n-1)p}\right)^2\right)\leq \exp\left(-\frac{k-1}{2}\cdot\left(1-\frac{k}{np}\right)^2\right).
 \end{align*}
Here we use the fact that if $k \in [n]$ and $p\in [k/n,1]$ then $k-1 \in [n-1]$ and $p \in [(k-1)/(n-1),1]$. We deduce further that
\begin{align*}
\Prob_{\sample_{n}}\left[ \rho\left(X_n,X_{\tau_{n,k}(x)}\right) > r_p(X_n)\right]&=\Prob_{\sample_{n}}\left[ \sum_{i \in [n]}\one\left\lbrace \dist\left(X_n,X_i \right)\leq r_p(X_n)\right\rbrace  < k\right]\\
&=\Prob_{\sample_{n}}\left[ \sum_{i \in [n-1]}\one\left\lbrace \dist\left(X_n,X_i \right)\leq r_p(X_n)\right\rbrace  < k-1\right]\\
&=\int_{\X} \Prob_{\sample_{n-1}}\left[ \sum_{i \in [n-1]}\one\left\lbrace \dist\left(x,X_i \right)\leq r_p(x)\right\rbrace  < k-1\right] d\marginalDistribution(x)\\
&\leq \exp\left(-\frac{k-1}{2}\cdot\left(1-\frac{k}{np}\right)^2\right).
\end{align*}
Hence, the bound also holds in case (b). This completes the proof of the lemma.
\end{proof}
