# Supplementary material for: Classification with unknown class-conditional label noise on non-compact feature spaces
Source: arXiv:1902.05627 source file (2019-06-09)
Supplement: Supplementary file 4 [file elementaryLemma.tex]

\begin{lemma}\label{elementaryRatioLemma} Suppose that $\estProbFlipZeroToOne, \estProbFlipOneToZero \in \left[0,1\right)$ with $\estProbFlipZeroToOne+\estProbFlipOneToZero<1$. Let $\noisy[{\est[\regressionFunction]}]:\X \rightarrow [0,1]$ be an estimate of $\noisyRegressionFunction$ and define $\est[\regressionFunction] :\X \rightarrow [0,1]$ by $\est[\regressionFunction](x):= \left(\noisy[{\est[\regressionFunction]}](x)-\estProbFlipZeroToOne\right)/\left(1-\estProbFlipZeroToOne-\estProbFlipOneToZero\right)$. Suppose that $\probFlipZeroToOne+\probFlipOneToZero<1$ and $\max\left\lbrace\left| \estProbFlipZeroToOne-\probFlipZeroToOne \right|, \left| \estProbFlipOneToZero-\probFlipOneToZero \right| \right\rbrace  \leq \left(1-\probFlipZeroToOne-\probFlipOneToZero\right)/4$. Then for all $x \in \X$ we have
\begin{align*}
\left| \est[\regressionFunction](x)-\regressionFunction(x)\right| \leq 6 \cdot \left(1-\probFlipZeroToOne-\probFlipOneToZero\right)^{-2} \cdot \max\left\lbrace \left| \estNoisyRegressionFunction(x) - \noisyRegressionFunction(x)\right|, \left| \estProbFlipZeroToOne-\probFlipZeroToOne \right|, \left| \estProbFlipOneToZero-\probFlipOneToZero \right| \right\rbrace.
\end{align*}
\end{lemma}
\begin{proof}
An elementary computation shows that given $\hat{a},a \in [-1,1]$ and $\hat{b},b \in \left(0,\infty\right)$ with $\left|\hat{b}-b\right| \leq b/2$ we have
\begin{align*}
\left|\frac{\hat{a}}{\hat{b}}-\frac{a}{b}\right| \leq \frac{3}{b^2}\cdot \max\left\lbrace \left|\hat{a}-a\right|, \left|\hat{b}-b\right| \right\rbrace.
\end{align*}
The corollary now follows from $\noisyRegressionFunction(x) = \left(1-\probFlipZeroToOne-\probFlipOneToZero\right) \cdot \regressionFunction(x)+ \probFlipZeroToOne$ (see (\ref{noisyRegInTermsOfTrueRegEq})) by taking $\hat{a} = \est[\noisyRegressionFunction](x)-\estProbFlipZeroToOne$, $a =\noisyRegressionFunction(x)-\probFlipZeroToOne$, $\hat{b} = 1-\estProbFlipZeroToOne-\estProbFlipOneToZero$ and $b = 1-\probFlipZeroToOne-\probFlipOneToZero$.
\end{proof}
